# Supplementary material for: High order maximum principle preserving finite volume method for convection dominated problems
Source: arXiv:1404.4041 source file (2014-04-15)
Supplement: Supplementary file 1 [file Appendix_A.tex]

\section*{Appendix A}
\label{appendix A}

In this section we derive the MPP flux limiters for two-dimensional problem. The basic idea is the same as for one-dimensional problem, i.e., necessary conditions for the numerical solutions to satisfy maximum principle will be derived, based on similar inequalities as (\ref{max}) and (\ref{min}).

Before further discussion, we briefly review the finite volume scheme for two dimensional problem. Similarly as in one dimensional case, we integrate Equation (\ref{ad2}) over cell $I_{i,j}$ and divide it by $\triangle x \triangle y$, then we have
\begin{align}\label{2dint}
\frac{1}{\triangle x \triangle y} \frac{d}{dt} \int \int_{I_{i,j}} u dxdy + & \frac{1}{\triangle x \triangle y} \int_{y_{j-\frac{1}{2}}}^{y_{j+\frac{1}{2}}} f(u)|_{x_{i+\frac{1}{2}}}dy - \frac{1}{\triangle x \triangle y} \int_{y_{j-\frac{1}{2}}}^{y_{j+\frac{1}{2}}} f(u)|_{x_{i-\frac{1}{2}}}dy \nonumber \\
 + & \frac{1}{\triangle x \triangle y} \int_{x_{i-\frac{1}{2}}}^{x_{i+\frac{1}{2}}} g(u)|_{y_{j-\frac{1}{2}}}dx - \frac{1}{\triangle x \triangle y} \int_{x_{i-\frac{1}{2}}}^{x_{i+\frac{1}{2}}} g(u)|_{y_{j-\frac{1}{2}}}dx  \nonumber \\
=& \frac{1}{\triangle x \triangle y} \int_{y_{j-\frac{1}{2}}}^{y_{j+\frac{1}{2}}} a(u)_x|_{x_{i+\frac{1}{2}}}dy - \frac{1}{\triangle x \triangle y} \int_{y_{j-\frac{1}{2}}}^{y_{j+\frac{1}{2}}} a(u)_x|_{x_{i-\frac{1}{2}}}dy \nonumber \\
 + & \frac{1}{\triangle x \triangle y} \int_{x_{i-\frac{1}{2}}}^{x_{i+\frac{1}{2}}} b(u)_y|_{y_{j-\frac{1}{2}}}dx - \frac{1}{\triangle x \triangle y} \int_{x_{i-\frac{1}{2}}}^{x_{i+\frac{1}{2}}} b(u)_y|_{y_{j-\frac{1}{2}}}dx.
\end{align}
Denote $\frac{1}{\triangle x \triangle y} \int \int_{I_{i,j}} u dxdy$ with $\bar{u}_{i,j}$, then the corresponding numerical scheme is
\begin{align}\label{2dscheme}
\frac{d}{dt} \bar{u}_{i,j} + & \frac{1}{\triangle x} (\hat{f}_{i+\frac{1}{2},j}-\hat{f}_{i-\frac{1}{2},j})+ \frac{1}{\triangle y} (\hat{g}_{i,j+\frac{1}{2}}-\hat{g}_{i,j-\frac{1}{2}}) \nonumber \\
&=\frac{1}{\triangle x} (\widehat{(a_x)}_{i+\frac{1}{2},j}-\widehat{(a_x)}_{i-\frac{1}{2},j}) +  \frac{1}{\triangle y} (\widehat{(b_y)}_{i,j+\frac{1}{2}}-\widehat{(b_y)}_{i,j-\frac{1}{2}}).
\end{align}
where $\hat{f}_{i+\frac{1}{2},j}$ can be understood as the average of the flux function over the right boundary of cell $I_{i,j}$, and $\hat{g}_{i,j+\frac{1}{2}}, \widehat{(a_x)}_{i+\frac{1}{2},j}, \widehat{(b_y)}_{i,j+\frac{1}{2}}$ have similar meanings. Applying Gaussian quadrature integration rules to the integrals involved in (\ref{2dint}), we have
\begin{align}
&  \hat{f}_{i+\frac{1}{2},j} = \frac{1}{2} \underset{i_g}{\Sigma} \omega_{i_g} f(u_{i+\frac{1}{2},i_g}),\\
&  \hat{g}_{i,j+\frac{1}{2}} = \frac{1}{2} \underset{i_g}{\Sigma} \omega_{i_g} g(u_{i_g,j+\frac{1}{2}}),\\
&  \widehat{(a_x)}_{i+\frac{1}{2},j} = \frac{1}{2} \underset{i_g}{\Sigma} \omega_{i_g} a_x( u_{i+\frac{1}{2},i_g} ),\\
&  \widehat{(b_y)}_{i,j+\frac{1}{2}} = \frac{1}{2} \underset{i_g}{\Sigma} \omega_{i_g} b_y( u_{i_g,j+\frac{1}{2}} ),
\end{align}
where $\underset{i_g}{\Sigma}$ represents the summation over the Gaussian quadratures and $u_{i+\frac{1}{2},i_g},u_{i_g,j+\frac{1}{2}}$ are the approximate values to $u(x_{i+\frac{1}{2}},y_{i_g}),u(x_{i_g},y_{j+\frac{1}{2}})$, and can be reconstructed from $\{\bar{u}_{i,j}\}$.  Details of the reconstruction procedure can be found in Appendix A.

Hence after discretized temporally with TVD Runge-Kutta method in the way similar to the case for the one dimensional problem, the scheme (\ref{2dscheme}) becomes
\begin{equation}
u_{i,j}^{n+1}=u_{i,j}^n - \lambda_x(\hat{H}^{rk}_{i+\frac{1}{2},j}-\hat{H}^{rk}_{i-\frac{1}{2},j}) -\lambda_y(\hat{G}^{rk}_{i,j+\frac{1}{2}}-\hat{G}^{rk}_{i,j-\frac{1}{2}}),
\end{equation}
where $\lambda_x=\frac{\triangle t}{\triangle x}$ and $\lambda_y=\frac{\triangle t}{\triangle y}$, and
\begin{align}
& \hat{H}^{rk}_{i+\frac{1}{2},j}=\frac{1}{6}(\hat{f}_{i+\frac{1}{2},j}^n - \widehat{(a_x)}_{i+\frac{1}{2},j}^n) + \frac{1}{6}(\hat{f}_{i+\frac{1}{2},j}^1 - \widehat{(a_x)}_{i+\frac{1}{2},j}^1) + \frac{2}{3} (\hat{f}_{i+\frac{1}{2},j}^2 - \widehat{(a_x)}_{i+\frac{1}{2},j}^2),\\
& \hat{G}^{rk}_{i,j+\frac{1}{2}}=\frac{1}{6}(\hat{g}_{i+\frac{1}{2},j}^n - \widehat{(b_x)}_{i+\frac{1}{2},j}^n) + \frac{1}{6}(\hat{g}_{i+\frac{1}{2},j}^1 - \widehat{(b_x)}_{i+\frac{1}{2},j}^1) + \frac{2}{3} (\hat{g}_{i+\frac{1}{2},j}^2 - \widehat{(b_x)}_{i+\frac{1}{2},j}^2).
\end{align}
$\hat{H}^{rk}_{i+\frac{1}{2},j}$ and $\hat{G}^{rk}_{i,j+\frac{1}{2}}$ can be understood as the average integral of the numerical fluxes in the temporal direction.

Similarly as for the one dimensional case, we modify the fluxes as follows,
\begin{align}
& \tilde{H}^{rk}_{i+\frac{1}{2},j}=\theta_{i+\frac{1}{2},j} \hat{H}^{rk}_{i+\frac{1}{2},j} + (1-\theta_{i+\frac{1}{2},j}) \hat{h}_{i+\frac{1}{2},j}, \label{2dmax}\\
& \tilde{G}^{rk}_{i,j+\frac{1}{2}}=\theta_{i,j+\frac{1}{2}} \hat{G}^{rk}_{i,j+\frac{1}{2}}+ (1-\theta_{i,j+\frac{1}{2}}) \hat{g}_{i,j+\frac{1}{2}},  \label{2dmin}
\end{align}
where $\hat{h}_{i+\frac{1}{2},j}$ and $\hat{g}_{i,j+\frac{1}{2}}$ are low order monotone flux that satisfy maximum principle, so that
\begin{equation}\label{constraint}
u_m \le u_{i,j}^n - \lambda_x(\tilde{H}^{rk}_{i+\frac{1}{2},j}-\tilde{H}^{rk}_{i-\frac{1}{2},j}) -\lambda_y(\tilde{G}^{rk}_{i,j+\frac{1}{2}}-\tilde{G}^{rk}_{i,j-\frac{1}{2}}) \le u_M,
\end{equation}
with $u_m=\underset{x,y}{min} \ u_0(x,y)$ and $u_M=\underset{x,y}{max} \ u_0(x,y)$.

Introducing the notations
\begin{align}
&F_{i-\frac{1}{2},j}=\lambda_x (\hat{H}^{rk}_{i-\frac{1}{2},j}-\hat{h}_{i-\frac{1}{2},j}), \nonumber \\
&F_{i+\frac{1}{2},j}=-\lambda_x (\hat{H}^{rk}_{i+\frac{1}{2},j}-\hat{h}_{i+\frac{1}{2},j}), \nonumber \\
&F_{i,j-\frac{1}{2}}=\lambda_y (\hat{G}^{rk}_{i,j-\frac{1}{2}}-\hat{g}_{i,j-\frac{1}{2}}), \nonumber \\
&F_{i,j+\frac{1}{2}}=-\lambda_y (\hat{G}^{rk}_{i,j+\frac{1}{2}}-\hat{g}_{i,j+\frac{1}{2}}), \nonumber
\end{align}
and plugging the modified fluxes (\ref{2dmax}) and (\ref{2dmin}) into (\ref{constraint}), we have
\begin{align}
&\theta_{i+\frac{1}{2},j} F_{i+\frac{1}{2},j} + \theta_{i-\frac{1}{2},j} F_{i-\frac{1}{2},j} + \theta_{i,j+\frac{1}{2}} F_{i,j+\frac{1}{2}} + \theta_{i,j-\frac{1}{2}} F_{i,j-\frac{1}{2}} \le \Gamma_{i,j}^M,  \label{2dmax1}\\
&\theta_{i+\frac{1}{2},j} F_{i+\frac{1}{2},j} + \theta_{i-\frac{1}{2},j} F_{i-\frac{1}{2},j} + \theta_{i,j+\frac{1}{2}} F_{i,j+\frac{1}{2}} + \theta_{i,j-\frac{1}{2}} F_{i,j-\frac{1}{2}} \ge \Gamma_{i,j}^m, \label{2dmin1}
\end{align}
where
\begin{align}
& \Gamma_{i,j}^M = u_M - (u_{i,j} - \lambda_x(\hat{h}_{i+\frac{1}{2},j}-\hat{h}_{i-\frac{1}{2},j}) - \lambda_y(\hat{g}_{i,j+\frac{1}{2}} - \hat{g}_{i,j-\frac{1}{2}}) ) \ge 0, \\
& \Gamma_{i,j}^m = u_m - (u_{i,j} - \lambda_x(\hat{h}_{i+\frac{1}{2},j}-\hat{h}_{i-\frac{1}{2},j}) - \lambda_y(\hat{g}_{i,j+\frac{1}{2}} - \hat{g}_{i,j-\frac{1}{2}}) ) \le 0.
\end{align}
Similarly as in the one dimensional case, we need to find numbers $\Lambda_{L,i,j}, \Lambda_{R,i,j}, \Lambda_{D,i,j}, \Lambda_{U,i,j}$ such that if
\begin{equation}
(\theta_{i-\frac{1}{2},j}, \theta_{i+\frac{1}{2},j}, \theta_{i,j-\frac{1}{2}}, \theta_{i,j+\frac{1}{2}}) \in [0,\Lambda_{L,i,j}]\times [0,\Lambda_{R,i,j}]\times [0,\Lambda_{D,i,j}]\times [0,\Lambda_{U,i,j}],
\end{equation}
then (\ref{2dmax1}) and (\ref{2dmin1}) hold.

We do similar analysis as for the one dimensional case, and the results are listed in Table \ref{Lambdasmax} and Table \ref{Lambdasmin}. (In the table, $'+'$ means that the corresponding variable is positive ($>0$) and $'-'$ means that it's non-positive ($\le 0$). And $\mathbf{F}=(F_{i-\frac{1}{2},j},F_{i+\frac{1}{2},j},F_{i,j-\frac{1}{2}},F_{i,j+\frac{1}{2}})$.)

Both the cases for maximum value and minimum value should be considered, so the numbers $\Lambda_{L,i,j}, \Lambda_{R,i,j}, \Lambda_{D,i,j}, \Lambda_{U,i,j}$ are
\begin{equation}
\begin{cases}
\Lambda_{L,i,j}=min(\Lambda_{L,i,j}^M,\Lambda_{L,i,j}^m),\\
\Lambda_{R,i,j}=min(\Lambda_{R,i,j}^M,\Lambda_{R,i,j}^m),\\
\Lambda_{D,i,j}=min(\Lambda_{D,i,j}^M,\Lambda_{D,i,j}^m),\\
\Lambda_{U,i,j}=min(\Lambda_{U,i,j}^M,\Lambda_{U,i,j}^m).
\end{cases}
\end{equation}
Finally we define the local limiter parameters as
\begin{equation}
\begin{cases}
\theta_{i+\frac{1}{2},j}=min(\Lambda_{R,i,j},\Lambda_{L,i+1,j}), \\
\theta_{i,j+\frac{1}{2}}=min(\Lambda_{U,i,j},\Lambda_{D,i,j+1}).
\end{cases}
\end{equation}
With these limiters, the numerical solution at each time step will satisfy the maximum principle. We will demonstrate the results in Section \ref{sec4}.

Given cell averages $\{ \bar{u}_{i,j} \}$, we need to reconstruct $u_{i+\frac{1}{2},i_g}$, the value of $u$ at $(x_{i+\frac{1}{2}},y_{i_g})$ where $y_{i_g}$ is the $i_g$-th Gaussian quadrature point on the interval $[y_{j-\frac{1}{2}},y_{j+\frac{1}{2}}]$.

To reconstruct $u_{i+\frac{1}{2},i_g}$, we consider $P(x)=u_(x,y_{i_g})$, then $u_{i+\frac{1}{2},i_g}=P(x_{i+\frac{1}{2}})$ and
\begin{equation}
\frac{1}{\triangle x} \int_{x_{i-\frac{1}{2}}}^{x_{i+\frac{1}{2}}} P(x)dx = \frac{1}{\triangle x} \int_{x_{i-\frac{1}{2}}}^{x_{i+\frac{1}{2}}} u_(x,y_{i_g})dx.
\end{equation}
So as long as we have $\frac{1}{\triangle x} \int_{x_{i-\frac{1}{2}}}^{x_{i+\frac{1}{2}}} u_(x,y_{i_g})dx$, the averages of $u(x,y)$ over the segments $\{ x\in [x_{i-\frac{1}{2}}, x_{i+\frac{1}{2}}], y=y_{i_g}\}$, then we can reconstruct $u_{i+\frac{1}{2},i_g}$ in the same way as in [ref]. So it suffices to reconstruct $\frac{1}{\triangle x} \int_{x_{i-\frac{1}{2}}}^{x_{i+\frac{1}{2}}} u_(x,y_{i_g})dx$. To do this, we consider $Q(y)=\frac{1}{\triangle x} \int_{x_{i-\frac{1}{2}}}^{x_{i+\frac{1}{2}}} u_(x,y))dx$, then $\frac{1}{\triangle x} \int_{x_{i-\frac{1}{2}}}^{x_{i+\frac{1}{2}}} u_(x,y_{i_g})dx=Q(y_{i_g})$ and
\begin{equation}
\frac{1}{\triangle y} \int_{y_{j-\frac{1}{2}}}^{y_{j+\frac{1}{2}}} Q(y)dy =\frac{1}{\triangle y} \frac{1}{\triangle x} \int_{x_{i-\frac{1}{2}}}^{x_{i+\frac{1}{2}}} u_(x,y))dx dy =\bar{u}_{i,j}.
\end{equation}
So $\frac{1}{\triangle x} \int_{x_{i-\frac{1}{2}}}^{x_{i+\frac{1}{2}}} u_(x,y_{i_g})dx$ can be reconstructed from cell averages $\{ \bar{u}_{i,j}\}$ with the method in [ref]. If we denote the standard reconstructing procedure in [ref] by $\mathcal{R}$, then the whole two dimensional finite volume reconstructing procedure can be illustrated as
\begin{equation}
\centering
\{ \bar{u}_{i,j}\} \overset{\mathcal{R}}{\longrightarrow}  \{\frac{1}{\triangle x} \int_{x_{i-\frac{1}{2}}}^{x_{i+\frac{1}{2}}} u_(x,y_{i_g})dx \} \overset{\mathcal{R}}{\longrightarrow} \{u_{i+\frac{1}{2},i_g}\}.
\end{equation}
